# Supplementary material for: Sparse Gaussian Process Variational Autoencoders
Source: arXiv:2010.10177 source file (2020-10-23)
Supplement: Supplementary file 1 [file old_appendix.tex]

\section{Mathematical Derivations}
\label{appendix:mathematical_derivations}
\subsection{Posterior Gaussian Process}
\label{appendix:posterior_gp}
For the sake of notation convenience, we shall drop the subscript $k$ from this derivation. Recall the approximate posterior over the inducing points, $\*u$:
\begin{equation}
    \qu = \frac{1}{\Zq} \underbrace{\normaldist{\*u}{\*0}{\Kuu}}_{\pu} \underbrace{\normaldist{\*u}{\luymu}{\luycov}}_{\luy}.
\end{equation}
$\qu$ is a Gaussian with mean and covariance given by
\begin{gather}
        \qfmu = \Kuu\suminv{\Kuu}{\luycov}\luymu \label{eq:qf_mu}\\
        \qfcov = \Kuu\suminv{\Kuu}{\luycov}\luycov = \suminv{\Kuu^{-1}}{\luycov^{-1}}. \label{eq:qf_cov}
\end{gather}
The approximate posterior over some latent function value $f_*$ is obtained by marginalisation of the joint distribution:
\begin{equation}
\begin{aligned}
    q(f_*) &= \int p_{\theta_1}(f_* | \*u) q(\*u) d\*u \\
    &= \int \normaldist{f_*}{k_{f_*\*u}\Kuu^{-1}\*u}{k_{f_*f_*} - k_{f_*\*u}\Kuu^{-1}k_{\*u f_*}} \normaldist{\*u}{\qfmu}{\qfcov} d\*u \\
    &= \normaldist{f_*}{k_{f_*\*u}\Kuu^{-1}\qfmu}{k_{f_*f_*} - k_{f_*\*u}\left(\Kuu^{-1} - \Kuu^{-1}\qfcov\Kuu^{-1}\right)^{-1}k_{\*u f_*}}.
\end{aligned}
\end{equation}
Substituting \eqref{eq:qf_mu} into the expression for the mean above gives rise to the GP mean function:
\begin{equation}
    \qgpmean{\*x} = \kfu\suminv{\Kuu}{\luycov}\luymu.
\end{equation}
The covariance function is a little trickier. First, expanding the matrix $\Kuu^{-1} - \Kuu^{-1}\qfcov\Kuu^{-1}$ using \eqref{eq:qf_cov} gives
\begin{equation}
\label{eq:covar_intermediate}
    \Kuu^{-1} - \Kuu^{-1}\qfcov\Kuu^{-1} = \Kuu^{-1} - \Kuu^{-1}\suminv{\Kuu^{-1}}{\luycov^{-1}}\Kuu^{-1}.
\end{equation}
Now we can apply the matrix inversion lemma to the right hand side of \eqref{eq:covar_intermediate} to give
\begin{equation}
    \Kuu^{-1} - \Kuu^{-1}\suminv{\Kuu^{-1}}{\luycov^{-1}}\Kuu^{-1} = \suminv{\Kuu}{\luycov}.
\end{equation}
Substituting this into the expression for the covariance gives rise to the GP covariance function:
\begin{equation}
    \qgpcov{\*x}{\*x'} = \kff - \kfu\suminv{\Kuu}{\luycov}\kuf.
\end{equation}

\subsection{Expectation of the Approximate Likelihood}
\label{appendix:expectation_approx_likelihood}
The quantity $\expectargs{\qu}{\log \luy}$ involves only the first and second moments of $\qu$ and so a closed form solution exists. Let $\*w_{nm}$ represent the concatenation of the difference in input locations, $\*z_{m} - \*x_n$, and output $\*y^o_n$. We have
\begin{align}
\label{eq:gpvae_luy_analytic_solution}
    \expectargs{\qu}{\log\luy} &= \sum_{k=1}^K \sum_{n=1}^N \sum_{m \in \mathcal{T}_n} \expectargs{\qumk}{\log\lumkwnm} \nonumber \\
    %
    &= \sum_{k=1}^K \sum_{n=1}^N \sum_{m \in \mathcal{T}_n} \expectargs{\qumk}{-\frac{(u_{mk} - \mu_{\phi, k}(\*w_{nm}))^2}{2\sigma^2_{\phi, k}(\*w_{nm})} - \frac{1}{2}\log |2\pi\sigma^2_{\phi, k}(\*w_{nm})|} \nonumber\\
    %
    &= \sum_{k=1}^K \sum_{n=1}^N \sum_{m \in \mathcal{T}_n} -\frac{\qfkcovm + (\qfkmum - \mu_{\phi, k}(\*w_{nm}))^2}{2\sigma^2_{\phi, k}(\*w_{nm})} - \frac{1}{2}\log |2\pi\sigma^2_{\phi, k}(\*w_{nm})| \nonumber \\
    %
    &= \sum_{k=1}^K \sum_{n=1}^N \sum_{m \in \mathcal{T}_n} \log \normaldist{\qfkmum}{\mu_{\phi, k}(\*w_{nm})}{\sigma^2_{\phi, k}(\*w_{nm})} - \frac{\qfkcovm}{2\sigma^2_{\phi, k}(\*w_{nm})} \nonumber \\
    %
    &= \sum_{k=1}^K \log \normaldist{\qfkmu}{\lfkymu}{\lfkycov} - \sum_{n=1}^N \frac{\qfkcovm}{2\sigma^2_{\phi, k}(\*w_{nm})}.
\end{align}

\subsection{Normalisation Constant}
\label{appendix:normalisation_constant}
First, note that each $\Zqk(\theta, \phi)$ can be re-written as a convolution between two Gaussians:
\begin{equation}
    \begin{aligned}
    \Zq(\theta, \phi) &= \prod_{k=1}^K \Zqk(\theta, \phi) = \prod_{k=1}^K \int \puk \luky d\*u_k \\
    &= \prod_{k=1}^K \int \normaldist{\*u_k}{\*0}{\Kukuk}\normaldist{\*u_k}{\lukymu}{\lukycov} d\*u_k \\
    &= \prod_{k=1}^K \int \normaldist{\*u_k}{\*0}{\Kukuk}\normaldist{\lukymu - \*u_k}{\*0}{\lukycov} d\*u_k.
    \end{aligned}
\end{equation}
The convolution between two Gaussians is also Gaussian, with mean and covariance given by the summation of the means and covariances of the original Gaussians. Thus, $\log \Zq(\theta, \phi)$ can be concisely expressed as
\begin{equation}
\label{eq:gpvae_zq_analytic_solution}
    \log \Zq(\theta, \phi) = \sum_{k=1}^K \underbrace{\log \normaldist{\lukymu}{\*0}{\Kukuk + \lukycov}}_{\log \Zqk(\theta, \phi)}.
\end{equation}

\subsection{Expectation of the Gradient of the Approximate Likelihood}
\label{appendix:expected_gradient_approx_likelihood}
The expected gradient of the approximate likelihood, $\expectargs{\qu}{\nabladot \log\luy}$, can be evaluated analytically as follows. Let $\*w_{nm}$ represent the concatenation of the difference in input locations, $\*z_{m} - \*x_n$, and output $\*y^o_n$. First, we make the expansion
\begin{equation}
\begin{aligned}
    \expectargs{\qu}{\nabladot \log\luy} &= \sum_{n=1}^N \sum_{m\in \mathcal{T}_n} \sum_{k=1}^K \expectargs{q(u_{mk})}{\nabladot \log \lumkwnm} \\
    &\mkern-100mu = \sum_{n=1}^N \sum_{m\in \mathcal{T}_n} \sum_{k=1}^K \expectargs{q(u_{mk})}{\nabladot\left(-\log\sigma_{\phi, k}(\*w_{nm}) - \frac{1}{2\sigma^2_{\phi, k}(\*w_{nm}}\left(u_{mk} - \mu_{\phi, k}(\*w_{nm})\right)^2\right)}. \\
\end{aligned}
\end{equation}
Application of the chain rule gives
\begin{equation}
\begin{aligned}
    \expectargs{q(u_{mk})}{\nabladot \log \lumkwnm} &= -\nabladot\log\sigma_{\phi, k}(\*w_{nm}) \\
    %
    &\phantom{=} - \expectargs{q(u_{mk})}{\left(u_{mk} - \mu_{\phi, k}(\*w_{nm})\right)^2} \nabladot \left(\frac{1}{2\sigma^2_{\phi, k}(\*w_{nm})}\right) \\
    %
    &\phantom{=} + \frac{1}{2\sigma^2_{\phi, k}(\*w_{nm})}\expectargs{q(u_{mk})}{u_{mk} - \mu_{\phi, k}(\*w_{nm})}\nabladot \mu_{\phi, k}(\*w_{nm}).
\end{aligned}
\end{equation}
We can expand the expectation $\expectargs{q(u_{mk})}{\left(u_{mk} - \mu_{\phi, k}(\*w_{nm})\right)^2}$ as
\begin{equation}
\begin{aligned}
    \expectargs{q(u_{mk})}{\left(u_{mk} - \mu_{\phi, k}(\*w_{nm})\right)^2} &= \expectargs{q(u_{mk})}{\left(u_{mk} - \qfkmum\right)^2} + (\qfkmum - \mu_{\phi, k}(\*w_{nm}))^2 \\
    &= \qfkcovm + (\qfkmum - \mu_{\phi, k}(\*w_{nm}))^2
\end{aligned}
\end{equation}
giving
\begin{equation}
\begin{aligned}
    \expectargs{q(u_{mk})}{\nabladot \log \lumkwnm} &= -\nabladot\log\sigma_{\phi, k}(\*w_{nm}) - \\
    &\phantom{=} \left(\qfkcovm + (\qfkmum - \mu_{\phi, k}(\*w_{nm}))^2\right) \nabladot \left(\frac{1}{2\sigma^2_{\phi, k}(\*w_{nm})}\right) \\
    &\phantom{=} + \frac{1}{2\sigma^2_{\phi, k}(\*w_{nm})}\left(\qfkmum - \mu_{\phi, k}(\*w_{nm})\right)\nabladot \mu_{\phi, k}(\*w_{nm}).
\end{aligned}
\end{equation}

\section{Monte Carlo Variational Inference}
\label{appendix:mc_vi}
As discussed in \Secref{subsec:mc_vi}, there are two techniques which can be applied to form an unbiased Monte Carlo estimate of the gradient of the ELBO. The first uses the log-derivative trick, whereas the second employs the reparameterisation trick \citep{kingma2013auto}. We refer to these two flavours of estimators as the \textit{score function estimator} and the \textit{path derivative estimator}, respectively. 

\subsection{Score Function Estimators}
\label{appendix:score_function_estimators}
Application of the log-derivative trick to $\nabladot\expectargs{\qf}{\pyf}$ is straightforward, giving
\begin{equation}
    \nabladot\expectargs{\qf}{\pyf} = \sum_{n=1}^N \expectargs{\qfn}{\log\pynfn\nabladot\log \qfn} + \expectargs{\qfn}{\nabladot \log\pynfn}.
\end{equation}
With the derivative operator now inside the expectation, an unbiased Monte Carlo estimate can be made. We refer to this estimator used in conjunction with the gradients of the analytic solutions for $\log \Zq(\theta, \phi)$ and $\expectargs{\qu}{\luy}$ as the \textit{semi-analytic score function estimator}.

Alternatively, the log-derivative trick can also be applied to $\nabladot \expectargs{\qu}{\luy}$. Starting from the ELBO, we have:
\begin{align}
    \nabladot \elbo &= \nabladot \expectargs{q(\*f, \*u)}{\log\frac{\pyf}{\luy}} + \nabladot \log \Zq(\theta, \phi) \nonumber \\
    &= \nabladot \sum_{n=1}^N \expectargs{q(\*f_n, \*u)}{\log\frac{\pynofn}{\luyno}} + \nabladot \log \Zq(\theta, \phi) \nonumber \\
    &= \sum_{n=1}^N \biggl\{\expectargs{q(\*f_n, \*u)}{\log\frac{\pynofn}{\luyno}\nabladot \log q(\*f_n, \*u)} \nonumber \\
    &\phantom{= \sum_{n=1}^N \biggl(} + \expectargs{q(\*f_n, \*u)}{\nabladot\log\frac{\pynofn}{\luyno}}\biggr\} + \nabladot \log \Zq(\theta, \phi).
\end{align}
When $\luyno \approx \pynofn$, the stochasticity of a Monte Carlo estimate for the first term in the summation cancels. However, the same is not true for the second term as the gradients do not cancel in general. Thus, we can expect a reduction in variance by pulling out $\expectargs{\qu}{\nabladot \log\luyno}$ and using the analytic solution provided in Appendix \ref{appendix:mathematical_derivations}. Collectively, we refer to this estimator as the \textit{doubly-stochastic score function estimator}.

\subsection{Path Derivative Estimators}
\label{appendix:path_derivative_estimators}
Using the reparameterisation
\begin{equation}
    f_{nk} = g_{\theta, \phi}(\epsilon_{nk}) = \qfkmun + \qfkcovn^{\frac{1}{2}}\epsilon_{nk}
\end{equation}
where $\epsilon_{nk} \sim \normaldist{\epsilon_{nk}}{0}{1}$, the expected log-likelihood can be re-written as
\begin{equation}
    \expectargs{\qf}{\log\pyf} = \sum_{n=1}^N \expectargs{p(\*\epsilon_n)}{\log \pynofrepar}
\end{equation}
where $\*\epsilon_n = (\epsilon_{n1}, \epsilon_{n2}, \ldots, \epsilon_{nk})$. Since $p(\*\epsilon_n)$ is independent of $\theta$ and $\phi$, the derivative operator can be moved inside the expectation, yielding
\begin{align}
    \nabladot \expectargs{\qf}{\log\pyf} &= \sum_{n=1}^N \expectargs{p(\*\epsilon_n)}{\nabladot \log \pynofrepar} \nonumber \\
    &\mkern-72mu = \sum_{n=1}^N \biggl\{\mathbb{E}_{p(\*\epsilon_n)}\biggl[\underbrace{\nabladot \log \pynofn}_{\text{score function}}\biggr] + \mathbb{E}_{p(\*\epsilon_n)}\biggl[\underbrace{\nabla_{\*f_n} \log \pynofn \nabladot g_{\theta, \phi}(\*\epsilon_n)}_{\text{path derivative}}\biggr]\biggr\}.
\end{align}
Used in combination with the gradients of the analytic solutions for $\log\Zq(\theta, \phi)$ and $\expectargs{\qu}{\luy}$, we refer to the estimator as the \textit{semi-analytic path derivative estimator}.

As with the log-derivative trick, an alternative estimator is derived by applying the reparameterisation trick to $\nabladot \expectargs{\qu}{\luy}$. Starting from the ELBO, we have:
\begin{align}
    \nabladot\elbo &= \nabladot \expectargs{q(\*f, \*u)}{\log\frac{\pyf}{\luy}} + \nabladot \log \Zq(\theta, \phi) \nonumber \\
    &= \sum_{n=1}^N \biggl\{ \mathbb{E}_{\pepsilon}\biggl[\underbrace{\nabladot \log \frac{\pynofn}{\luyno}}_{\text{score function}}\biggr] + \mathbb{E}_{\pepsilon}\biggl[\underbrace{\nabla_{\*f_n}\log \frac{\pynofn}{\luyno}\nabladot g_{\theta, \phi}(\*\epsilon_n)}_{\text{path derivative}}\biggr]\biggr\} \nonumber \\
    &\phantom{=} + \nabladot\log\Zq(\theta, \phi).
\end{align}
Whereas the stochasticity of the path derivative term cancels when the approximate posterior is close to the true posterior, the stochasticity of the score function term does not. Similar to the doubly-stochastic score function estimator, we define the \textit{doubly-stochastic path derivative estimator} using analytical solutions for $\expectargs{\qu}{\nabladot \log\luyno}$ and $\log\Zq(\theta, \phi)$.


\section{Multi-Output Gaussian Processes}
\label{sec:multi_output_gps}
Through consideration of the interchange of input dependencies and likelihood functions, we can shed light on the relationship between the probabilistic model employed by the \model{} and other multi-output GP models. These relationships are summarised in \Figref{fig:multi_ouput_gps_unified}. 

\begin{figure}[h]
\centering
\begin{tikzpicture}
	\footnotesize
	
	% Cube colour.
	\colorlet{fc}{black!10}
      
	% Vanishing points for perspective handling.
	\coordinate (P1) at (-15cm,2cm); % left vanishing point
	\coordinate (P2) at (15cm,2cm); % right vanishing point

	% (A1) and (A2) defines the 2 central points of the cuboid.
	\coordinate (A1) at (0em,0cm); % central top point
	\coordinate (A2) at (0em,-3.33cm); % central bottom point

	% (A3) to (A8) are computed given a unique parameter (or 2) .8
	% You can vary .8 from 0 to 1 to change perspective on left side
	\coordinate (A3) at ($(P1)!.8!(A2)$); % To pick for perspective 
	\coordinate (A4) at ($(P1)!.8!(A1)$);

	% You can vary .8 from 0 to 1 to change perspective on right side
	\coordinate (A7) at ($(P2)!.8!(A2)$);
	\coordinate (A8) at ($(P2)!.8!(A1)$);

	% Automatically compute the last 2 points with intersections
	\coordinate (A5) at
	  (intersection cs: first line={(A8) -- (P1)},
			    second line={(A4) -- (P2)});
	\coordinate (A6) at
	  (intersection cs: first line={(A7) -- (P1)}, 
			    second line={(A3) -- (P2)});
	
% 	\draw[thick,dashed,opacity=0.5] (A5) -- (A6);
% 	\draw[thick,dashed,opacity=0.5] (A3) -- (A6);
% 	\draw[thick,dashed,opacity=0.5] (A7) -- (A6);
% 	\draw[thick,dashed,opacity=0.5] (A4) -- (A5);
% 	\draw[thick,dashed,opacity=0.5] (A8) -- (A5);

	\fill[fc,opacity=0.3] (A1) -- (A8) -- (A7) -- (A2) -- cycle; % right face
	\fill[fc,opacity=0.3] (A1) -- (A2) -- (A3) -- (A4) -- cycle; % left face
    \fill[fc,opacity=0.3] (A1) -- (A4) -- (A8) -- cycle; % top face
    \fill[fc,opacity=0.3] (A2) -- (A3) -- (A7) -- cycle; % bottom face
    \fill[fc,opacity=0.3] (A3) -- (A4) -- (A8) -- (A7) -- cycle; % middle face


	% Possibly draw front lines
	\draw[thick] (A1) -- (A2);
	\draw[thick] (A3) -- (A4);
	\draw[thick] (A7) -- (A8);
	\draw[thick] (A1) -- (A4);
	\draw[thick] (A1) -- (A8);
	\draw[thick] (A2) -- (A3);
	\draw[thick] (A2) -- (A7);

% 	\draw[thick] (A3) -- (A7);
	\draw[thick] (A4) -- (A8);
	
	% Annotated edges between coordinates.
	\path [every edge/.append style={thick, draw=black, ->, shorten >=.25cm,shorten <=.25cm, sloped,anchor=south}] 
% 	(A2) +(5pt,-5pt) coordinate (A2br) edge node[below,align=center,yshift=-5pt,xshift=5pt] {Linear likelihood} ([xshift=5pt,yshift=-5pt]A7)
% 	(A2) +(-5pt,-5pt) coordinate (A2bl) edge node[below,align=center,yshift=-5pt,xshift=-5pt] {GP likelihood} ([xshift=-5pt,yshift=-5pt]A3)
% 	(A4) +(-5pt,0) coordinate (A4bl) edge node[left,align=center,yshift=-20pt,xshift=30] {Remove input \\ dependencies} (A4bl |- A3);
% 	(A8) +(+5pt,0) coordinate (A8br) edge node[right,align=center,xshift=-30pt,yshift=15pt] {Remove input \\ dependencies} (A8br |- A7);
    (A1) +(7pt,-7pt) coordinate (A1br) edge node[below,align=center,yshift=0pt,xshift=2.5pt] {Linear likelihood} ([xshift=0pt,yshift=-7pt]A8)
	(A1) +(-7pt,-7pt) coordinate (A1bl) edge node[below,align=center,yshift=-0pt,xshift=-2.5pt] {GP likelihood} ([xshift=0pt,yshift=-7pt]A4)
    (A1) +(+5pt,0) coordinate (A1br) edge node[right,align=center,xshift=-30pt,yshift=15pt] {Remove input \\ dependencies} (A1br |- A2);
	
	% Draw black nodes.
	\foreach \i in {1,2,3,4,7,8}
	{
	  \draw[fill=black] (A\i) circle (0.25em);
	}
	
	% GP-VAE node.
    \draw(A1) node[above,text width=4cm,align=center,yshift=20pt] (gpvae) {\textbf{\model} \\[1.25ex] $f_k \sim \mathcal{GP}(0,\ k(\*x, \*x'))$ \\ $\*y_n|\*f_n \sim \mathcal{N}(\*\mu(\*f_n),\ \*\Sigma(\*f_n))$};
    
     % VAE node.
    \draw(A2) node[below,text width=4cm,align=center,yshift=-10pt] (vae) {\textbf{VAE} \\[1.25ex] $\*f_n \sim \mathcal{N}(\*0, \*I)$ \\ $\*y_n|\*f_n \sim \mathcal{N}(\*\mu(\*f_n),\ \*\Sigma(\*f_n))$};
    
    % GP-FA node.
    \draw(A8) node[right,text width=4cm,align=center,xshift=-10pt] (gpfa) {\textbf{GP-FA} \\[1.25ex] $f_k \sim \mathcal{GP}(0,\ k(\*x, \*x'))$ \\ $\*y_n|\*f_n \sim \mathcal{N}(\*W\*f_n,\ \*\Sigma)$};
    
    % Factor analysis node.
    \draw(A7) node[right,text width=4cm,align=center,xshift=-10pt] (fa) {\textbf{Factor Analysis} \\[1.25ex] $\*f_n \sim \mathcal{N}(\*0, \*I)$ \\ $\*y_n|\*f_n \sim \mathcal{N}(\*W\*f_n,\ \*\Sigma)$};
    
    % GP-LVM node.
    \draw(A3) node[left,text width=4cm,align=center,xshift=10pt] (gplvm) {\textbf{GP-LVM} \\[1.25ex] $\*f_n \sim \mathcal{N}(\*0,\ \*I)$ \\ $y_p|f \sim \mathcal{GP}(0,\ k(\*f,\*f'))$};
    
    % Deep GP node.
    \draw(A4) node[left,text width=4cm,align=center,xshift=10pt] (dgp) {\textbf{DGP} \\[1.25ex] $f_k \sim \mathcal{GP}(0,\ k(\*x,\*x')$ \\ $y_p|f \sim \mathcal{GP}(0,\ k(\*f,\*f'))$};
\end{tikzpicture}
\caption{A unifying perspective on multi-output GPs.}
\label{fig:multi_ouput_gps_unified}
\end{figure}

\textbf{Linear Multi-Output Gaussian Processes} Replacing the likelihood with a linear likelihood function characterises a family of linear multi-output GPs, defined by a linear transformation of $K$ independent latent GPs:
\begin{equation}
\begin{gathered}
    f \sim \prod_{k=1}^K \gaussianprocess{0}{k_{\theta_{1,k}}(\*x, \*x')} \\
    \*y | f \sim \prod_{n=1}^N \normaldist{\*y_n}{\*W\*f_n}{\*\Sigma}.
    \end{gathered}
\end{equation}
The family includes \possessivecite{seeger2005semiparametric} semiparametric latent factor model, \possessivecite{byron2009gaussian} GP factor analysis (GP-FA) and \possessivecite{bonilla2008multi} class of multi-task GPs. Notably, removing input dependencies by choosing $k_{\theta_{1,k}}(\*x, \*x') = \delta(\*x, \*x')$ recovers factor analysis, or equivalently, probabilistic principal component analysis \citep{tipping1999probabilistic} when $\*\Sigma = \sigma^2 \*I$. Akin to the relationship between factor analysis and linear multi-output GPs, the probabilistic model employed by standard VAEs can be viewed as a special, instantaneous case of the \model 's.

\textbf{Deep Gaussian Processes} Single hidden layer deep GPs (DGPs) \citep{damianou2013deep} are characterised by the use of a GP likelihood function, giving rise to the probabilistic model
\begin{equation}
\begin{gathered}
    f \sim \prod_{k=1}^K \gaussianprocess{0}{k_{\theta_{1,k}}(\*x, \*x')} \\
    y | f \sim \prod_{p=1}^P \gaussianprocess{0}{k_{\theta_{2,p}}(f(\*x) f(\*x'))}
\end{gathered}
\end{equation}
where $\*y_n = y(\*x_n)$. The GP latent variable model (GP-LVM) \citep{lawrence2007hierarchical} is the special, instantaneous case of single layered DGPs. Multi-layered DGPs are recovered using a hierarchical latent space with conditional GP priors between each layer. 

\section{Experimental Details}
\label{appendix:experimental_details}
Whilst the theory outlined in \Secref{sec:spatio_temporal_vae} describes a general decoder parameterising both the mean and variance of the likelihood, we experienced difficulty training \model s using a learnt variance, especially for high-dimensional observations. Thus, for the experiments detailed in this paper we use a shared variance across all observations. We use the Adam optimiser \citep{kingma2014adam} with a constant learning rate of 0.001. Unless stated otherwise, we estimate the gradients of the ELBO using a single sample and the ELBO itself, as well as the predictive distribution, using 100 samples. For each experiment, we normalise the observations using the means and standard deviations of the data in the training set.

The computational complexity of performing VI in the full GP-VAE is dominated by the $\order{KN^3}$ cost associated with inverting the set of $K$ $N\times N$ matrices, $\{\Kfkfk + \lfkycov\}_{k=1}^K$. This can quickly become burdensome for even moderately sized datasets. A pragmatic workaround is to use a biased estimate of the ELBO using $\tilde{N} < N$ data points:
\begin{equation}
    \tilde{\mathcal{L}}_{\textrm{ELBO}}^{\tilde{N}} = \frac{N}{\tilde{N}}\left[ \expectargs{q(\tilde{\*f})}{\log \frac{p_{\theta_2}(\tilde{\*y}|\tilde{\*f})}{l_{\phi}(\tilde{\*f} | \tilde{\*y})}} + \log \tilde{\Zq}(\theta, \phi)\right].
\end{equation}
$\tilde{\*y}$ and $\tilde{\*f}$ denote the mini-batch of $\tilde{N}$ observations and their corresponding latent variables, respectively. The bias is introduced due to the normalisation constant, which does not satisfy $\frac{N}{\tilde{N}} \expectargs{}{\log \tilde{\Zq}(\theta, \phi)} = \expectargs{}{\log \Zq(\theta, \phi)}$. Nevertheless, the mini-batch estimator will be a reasonable approximation to the full estimator provided the lengthscale of the GP prior is not too large.\footnote{In which case the off-diagonal terms in the covariance matrix will be large making the approximation $\pf = \prod p_{\theta_1}(\tilde{\*f)}$ extremely crude.} We emphasise that mini-batching cannot be used to reduce the $\order{KN^3}$ cost of performing inference at test time, hence sparse approximations are necessary for large datasets.

\subsection{Small-Scale EEG}
For all GP-VAE models, we use a three-dimensional latent space, each using squared exponential (SE) kernels with lengthscales and scales initialised to 0.1 and 1, respectively. All DNNs, except for those in PointNet and IndexNet, use two hidden layers of 20 units and ReLU activation functions. PointNet and IndexNet employ DNNs with a single hidden layer of 20 units and a 20-dimensional intermediate representation. Each model is trained for 3000 epochs using a batch size of 100, with the procedure repeated 15 times. Following \citep{requeima2019gaussian}, the performance of each model is evaluated using the standardised mean squared error (SMSE) and negative log-likelihood (NLL). The mean $\pm$ standard deviation of the performance metrics for the 10 iterations with the highest ELBO is reported.\footnote{We found that the GP-VAE occasionally got stuck in very poor local optima. Since the ELBO is calculated on the training set alone, the experimental procedure is still valid.}

\subsection{Jura}
We use a two-dimensional latent space for all GP-VAE models with SE kernels with lengthscales and scales initialised to 1. Similar to the EEG data imputation task, using fewer latent dimensions than observed dimensions forces the model to share information across dimensions. Furthermore, this permits a fair comparison with other multi-output GP methods which also use two latent dimensions with SE kernels. For all DNNs except for those in IndexNet, we use two hidden layers of 20 units and ReLU activation functions. IndexNet uses DNNs with a single hidden layer of 20 units and a 20-dimensional intermediate representation. Following \cite{goovaerts1997geostatistics} and \cite{lawrence2004gaussian}, the performance of each model is evaluated using the mean absolute error (MAE) averaged across 10 different initialisations. The 10 different initialisations are identified from a body of 15 as those with the highest training set ELBO. For each initialisation the GP-VAE models are trained for 3000 epochs using a batch size of 100.

\subsection{Large-Scale EEG}
For each trial in the test set, we simulate simultaneous electrode `blackouts' by removing any 4 sample period at random with 25\% probability. Additionally, we simulate individual electrode `blackouts' by removing any 16 sample period at random with 25\% probability for both the training and test set. All models are trained for 100 epochs, with the procedure repeated five times, and use a 10-dimensional latent space with SE kernels and lengthscales initialised to 1 and 0.1, respectively. All DNNs, except for those in PointNet and IndexNet, use four hidden layers of 50 units and ReLU activation functions. PointNet and IndexNet employ DNNs with two hidden layers of 50 units and a 50-dimensional intermediate representation. For the \model, we place fixed inducing points every four samples with the inference network parameterising the nearest one. 

\subsection{Bouncing Ball}
To ensure a fair comparison with the SVAE and SIN, we adopt an identical architecture for the inference network and decoder in the original experiment. In particular, we use DNNs with two hidden layers of 50 units and hyperbolic tangent activation functions. Whilst both \citeauthor{johnson2016composing} and \citeauthor{lin2018variational} use eight-dimensional latent spaces, we consider a GP-VAE with a one-dimensional latent space and periodic GP kernel. For the more complex experiment, we use a \model{} with fixed inducing points placed every 10 samples and an inference network parameterising the nearest one. We also increase the number of hidden units in each layer of the DNNs to 128 and use a two-dimensional latent space - one for each ball. 

\subsection{Weather Station}
The spatial location of each weather station is determined by its latitude, longitude and elevation above sea level. The rates of missingness in the dataset vary, with 6.3\%, 14.0\%, 18.9\%, 47.3\% and 93.2\% of values missing for each of the five weather variables, respectively. Each model is trained on the data from 1980 using a single group per update for 25 epochs, with the performance evaluated on the data from both 1980 and 1981 using the root mean squared error (RMSE) and NLL averaged across five runs. We use a three-dimensional latent space with SE kernels and lengthscales initialised to 1. All DNNs, except for those in PointNet and IndexNet, use four hidden layers of 50 units and ReLU activation functions. PointNet and IndexNet employ DNNs with two hidden layers of 50 units and a 50-dimensional intermediate representation. Inducing point locations are initialised using k-means clustering, and are shared across each dimension and group. The VAE uses IndexNet. No comparison to other sparse GP approaches is made and there is no existing framework for performing approximate inference in sparse GP models conditioned on previously unobserved data. 

\section{Further Experimentation}
\label{appendix:further_experimentation}

\subsection{Comparing Estimators}
\label{appendix:comparing_estimators}
\subsubsection{Gradient Estimators}
\label{appendix:comparing_gradient_estimators}
In Appendix \ref{appendix:mc_vi}, four methods for estimating the gradients of the ELBO for the \model{} were presented: the semi-analytic score function estimator (SA-SF), the doubly-stochastic score function estimator (DS-SF), the semi-analytic path derivative estimator (SA-PD) and the doubly-stochastic path derivative estimator (DS-PD). To compare the effectiveness of each, we consider the task of modelling a toy dataset composed of samples from four interdependent functions: 
\begin{align*}
    y_1(x) &= 2\sin(0.2x) - 0.5\cos(x) \\
    y_2(x) &= 2\cos(0.5x) + 2\sin(0.1x) - 5 \\
    y_3(x) &= -y_1(x) + 3y_2(x) \\
    y_4(x) &= 0.5y_1(x) -2y_2(x).
\end{align*}

In each case, a two-dimensional latent space with SE kernels is used. All lengthscales and output scales are initialised to 1 and all DNNs are composed of two hidden layers of 20 units with ReLU activation functions. A dataset of 100 data points is formed by sampling each of the four functions uniformly in the range $x \in \left[-50, 150\right]$. 

\begin{figure}[ht]
    \centering
    \includegraphics[width=\textwidth]{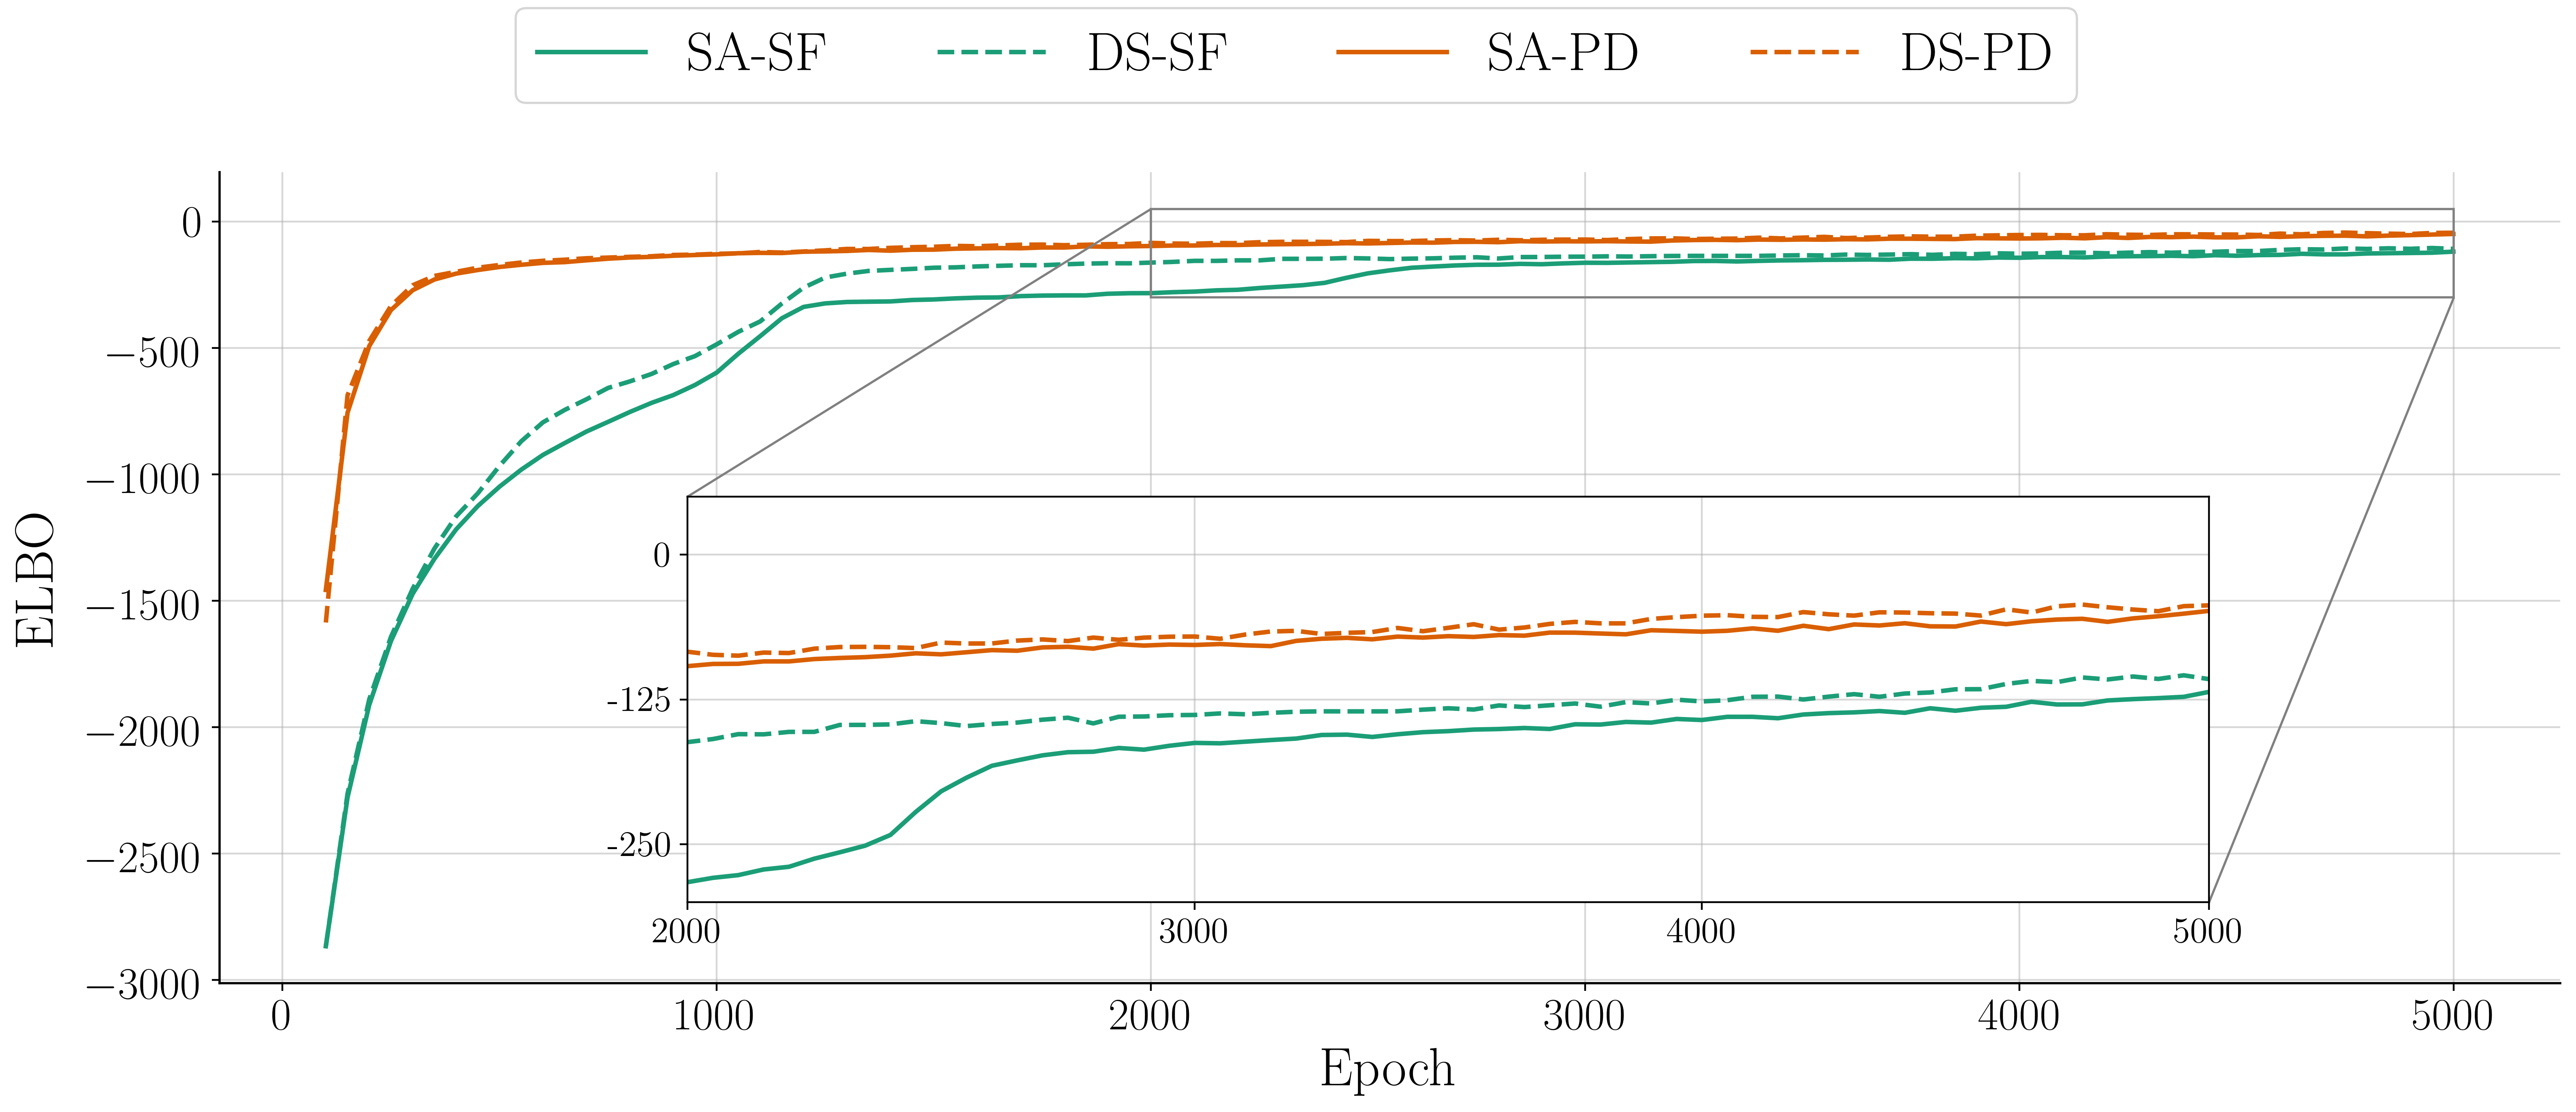}
    \caption[A comparison between ELBO gradient estimators.]{A comparison between the GP-VAE ELBO when trained using each of the four estimators: semi-analytic score function (SA-SF), doubly-stochastic score function (SF), semi-analytic path derivative (SA-PD) and doubly-stochastic path derivative (PD).}
    \label{fig:elbo_grad_comparison}
\end{figure}

Figure \ref{fig:elbo_grad_comparison} compares the progression of the ELBO for GP-VAEs optimised using each of the four estimators. In agreement with the results of others, the path derivative estimators outperform the score function estimators for the entirety of training. Observe that the doubly-stochastic estimators result in marginally faster training than the semi-analytic estimators. As previously discussed in \Secref{subsec:mc_vi}, this suggests that stochasticity of the Monte Carlo estimates cancels, which in turn, suggests that the quality of the approximate posterior is good.

\subsubsection{ELBO Estimators}
\label{appendix:comparing_elbo_estimators}
Figure \ref{fig:elbo_comparison} compares the empirical variance of the semi-analytic ELBO estimator (SA-ELBO) and doubly-stochastic ELBO (DS-ELBO) estimator using a single sample. 

\begin{figure}[ht]
    \centering
    \includegraphics[width=1.\textwidth]{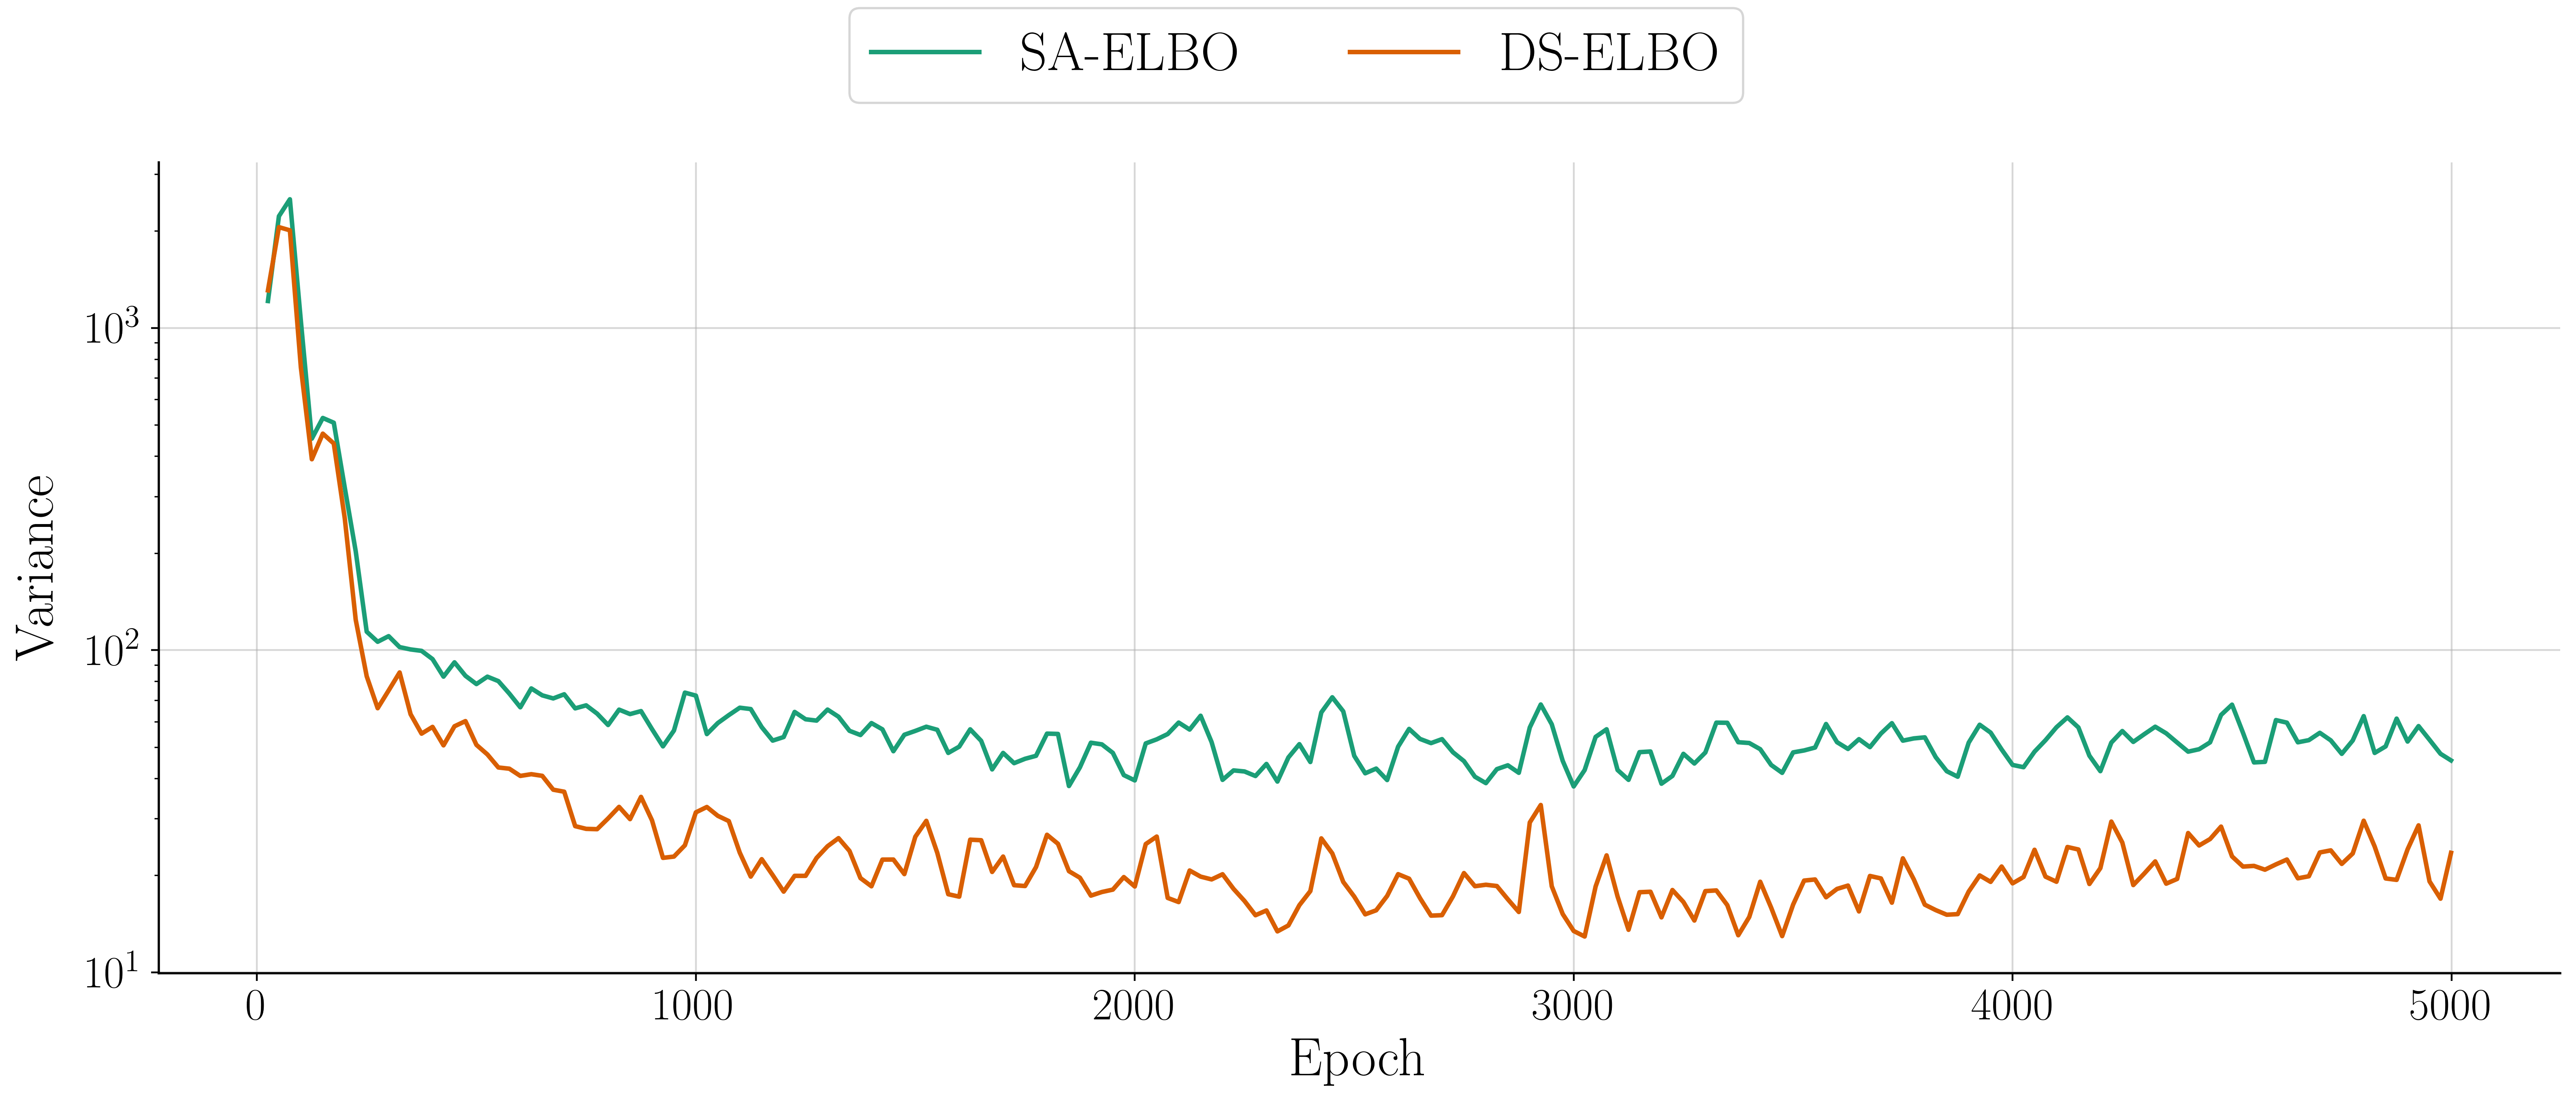}
    \caption[A comparison between ELBO estimators.]{A comparison between the variance of the semi-analytic ELBO estimator (SA-ELBO) and doubly-stochastic ELBO estimator (DS-ELBO) for the GP-VAE trained on the toy dataset using the DS-PD estimator.}
    \label{fig:elbo_comparison}
\end{figure}

Similar to \ref{fig:elbo_grad_comparison}, we see that the doubly-stochastic estimator has a stronger empirical performance than its semi-analytic counterpart, consistent with the claim that the quality of the approximate posterior is good. Observe that the difference between the variance of the estimators sharply increases in synchrony with the increase in ELBO shown in Figure \ref{fig:elbo_grad_comparison}. The increase in ELBO is due to the approximate posterior improving, which results in a reduction in stochasticity of the doubly-stochastic estimators.

\subsection{Bouncing Ball Experiment}
\label{appendix:bouncing_ball_experiment}
The original dataset consists of 80 12-dimensional image sequences each of length 50, with the task being to predict the trajectory of the ball given a prefix of a longer sequence. The image sequences are generated at random by uniformly sampling the starting position of the ball whilst keeping the bouncing frequency fixed. \Figref{fig:bb_linear_dynamics} compares the posterior latent GP and mean of the posterior predictive distribution with the ground truth for a single image sequence using just a single latent dimension. As demonstrated in the more more complex experiment, the GP-VAE is able to recover the ground truth with almost exact precision.

\begin{figure}[ht]
    \centering
    \includegraphics[width=\textwidth]{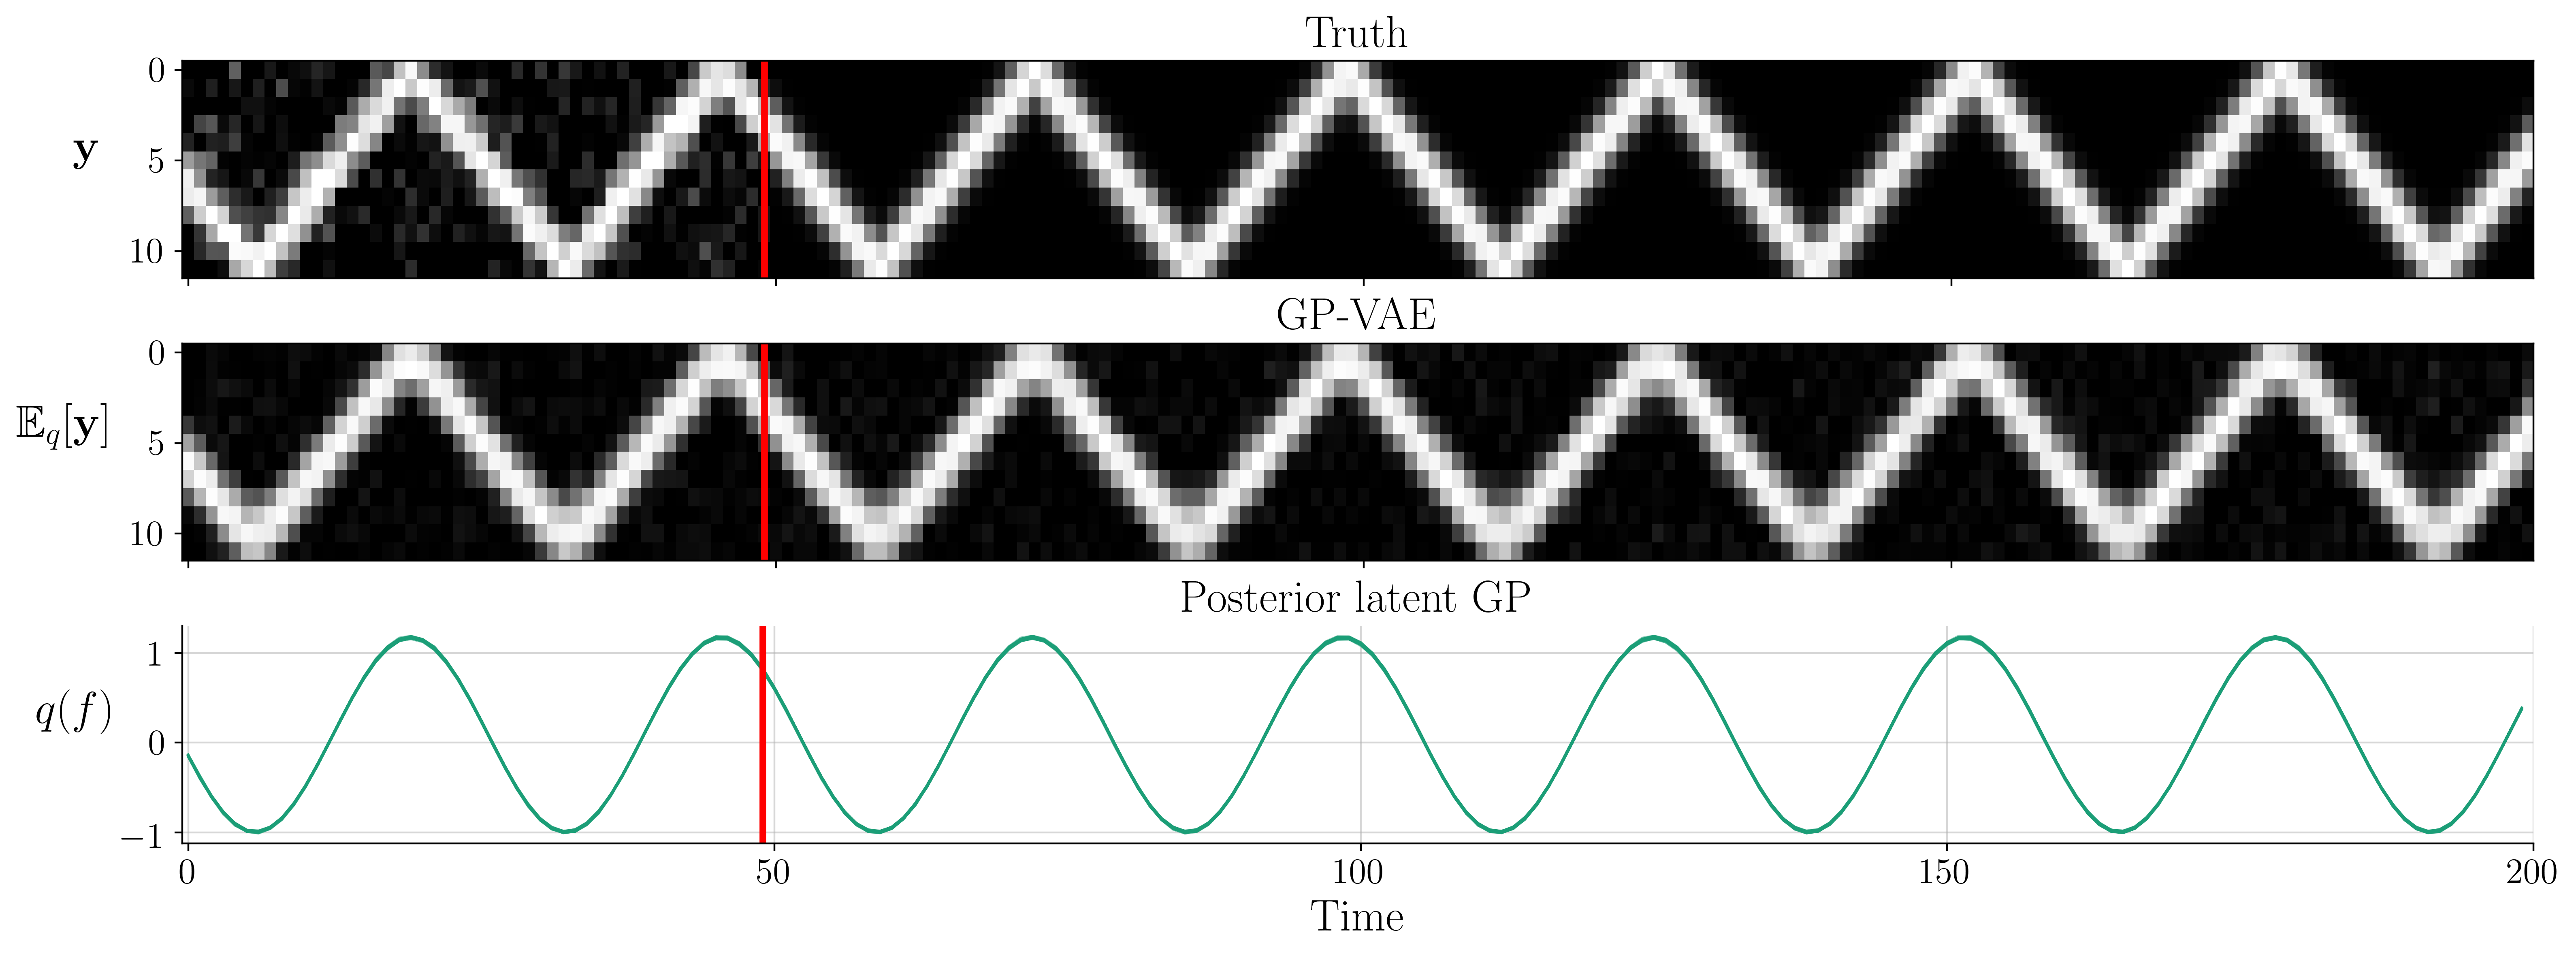}
    \caption[The posterior predictive distribution of the GP-VAE on the bouncing ball dataset.]{A comparison between the mean of the GP-VAE's posterior predictive distribution (middle) and the ground truth (top) conditioned on noisy observations up to the red line. The latent approximate GP posterior is also shown (bottom).}
    \label{fig:bb_linear_dynamics}
\end{figure}

Following \cite{lin2018variational}, we evaluate the $\tau$-steps ahead predictive performance of the \model{} using the mean absolute error, defined as
\begin{equation}
    \sum_{n=1}^{N_{\text{test}}} \sum_{t=1}^{T-\tau} \frac{1}{N_{\text{test}}(T-\tau)d} \left\|\*y^*_{n, t+\tau} - \expectargs{q(y_{n, t+\tau}|y_{n, 1:t})}{\*y_{n, t+\tau}}\right\|_1
\end{equation}
where $N_{\text{test}}$ is the number of test image sequences with $T$ time steps and $\*y^*_{n, t+\tau}$ denotes the noiseless observation at time step $t+\tau$. \Figref{fig:bb_mean_prediction_error} compares the performance of the \model{} with the SVAE and SIN using LDS priors, alongside the benchmark performance of the regular LDS. Despite using just a single latent dimension, the \model{} significantly outperforms the other two structured VAE models.

\begin{figure}[ht]
    \centering
    \includegraphics[width=0.8\textwidth]{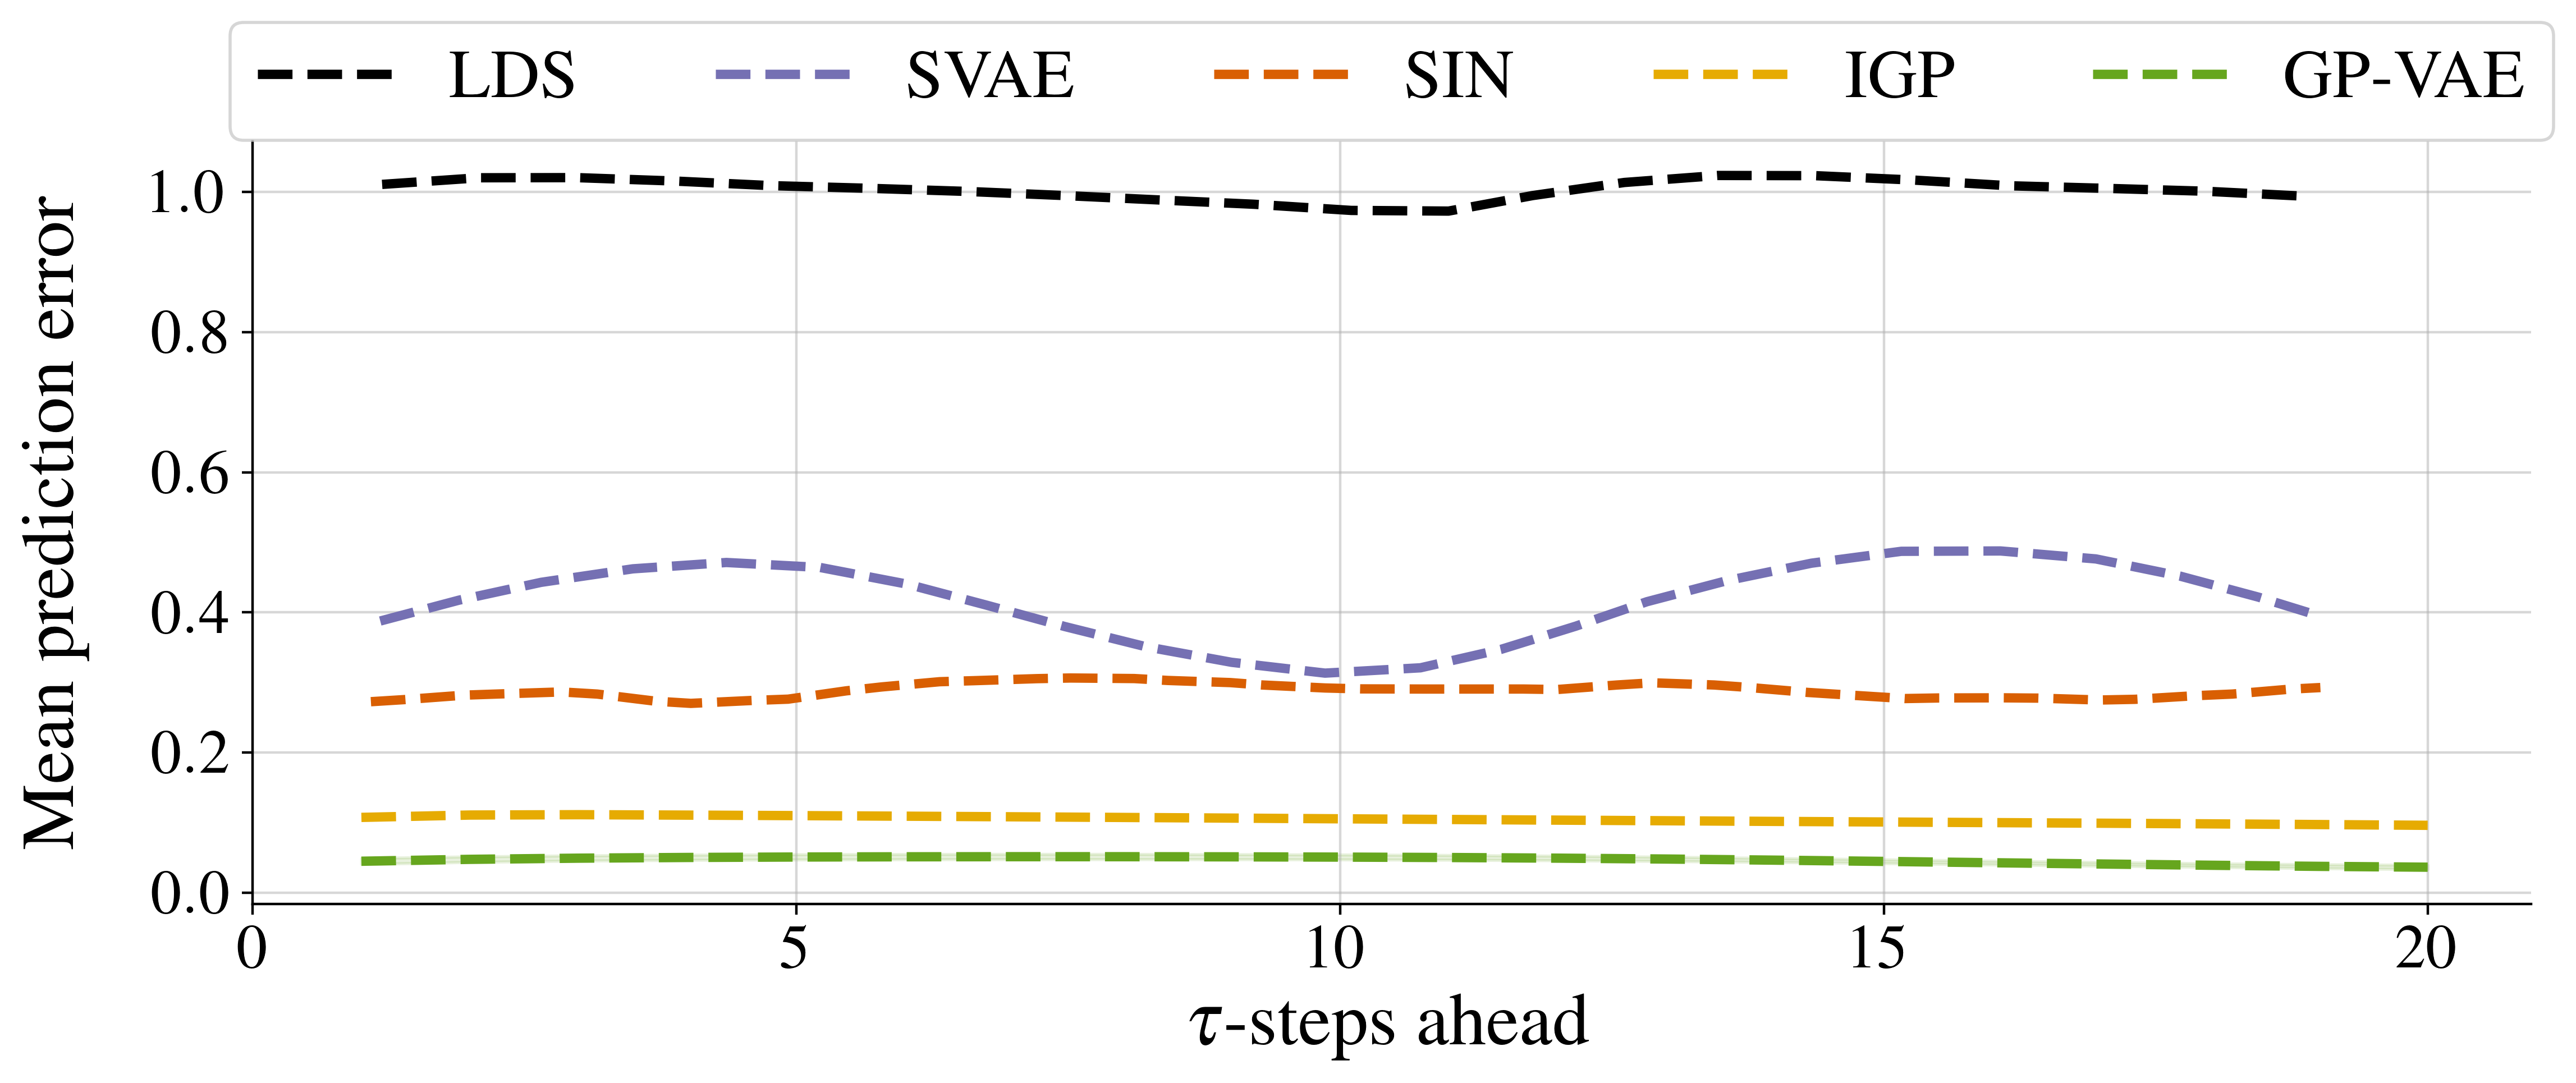}
    \caption[A comparison between the predictive performance of the GP-VAE relative to the SVAE and SIN on the bouncing ball experiment.]{A comparison between the $\tau$-steps ahead predictive performance of the GP-VAE, SVAE, SIN and regular LDS. For the GP-VAE the mean $\pm$ standard deviation is shown. The results for the SVAE, SIN and regular LDS are taken directly from \cite{lin2018variational}.}
    \label{fig:bb_mean_prediction_error}
\end{figure}
